# Supplementary material for: Channel flows of deformable nematics
Source: arXiv:2508.19013 ancillary file (2025-08-26)
Supplement: Supplementary file 1 [file Supplementary_Material.pdf]

# Electronic Supplementary Material
# Channel flows of deformable nematics

Ioannis Hadjifrangiskou[1], Sumesh P. Thampi[1,2], and Julia M. Yeomans[1]

[1]Rudolf Peierls Centre for Theoretical Physics, University of Oxford, Oxford OX1 3PU, United Kingdom

[2]Department of Chemical Engineering, Indian Institute of Technology Madras, Chennai-36, India

## 1 Movie 1

Animation of deformable particles in an imposed Couette flow for $\alpha = 1, \xi_0 = 1$ showing shape oscillations, corresponding to region I in Fig. 1. Vector field indicates the imposed Couette flow. Solid black lines indicate channel walls.

## 2 Movie 2

Animation of deformable particles in an imposed Poiseuille flow for $\beta = 0$. The spatially dependent shear rate leads to shape oscillations near the channel centre and a steady flow-aligned configuration near the channel walls. Vector field indicates the imposed flow. Brown dashed lines indicate the boundary between the regions exhibiting shape oscillations, and those that reach a flow-aligned steady state. Solid black lines indicate channel walls.

## 3 Characteristic dynamics of deformable nematics in a Couette flow

### 3.1 Time period of shape oscillations in regions I and II

The time period of shape oscillations of deformable particles subjected to a Couette flow depends on the applied shear rate (or Péclet number), $\alpha$, and the flow alignment scale, $\xi_0$. While the system is in region I (see Fig. 1), the time period of the shape oscillations decreases with an increase in the shear rate, $\alpha$, and mildly increases with an increase in the flow alignment scale, $\xi_0$, as shown in Fig. S1. In region II, however, increasing $\alpha$ or $\xi_0$ further allows the limit cycle trajectory in phase space to approach the saddle point. Consequently, the system enters a ghost region [1] in the phase space where the dynamics slow down considerably. In particular, the period of oscillations diverges as the system gets arbitrarily close to the homoclinic bifurcation.

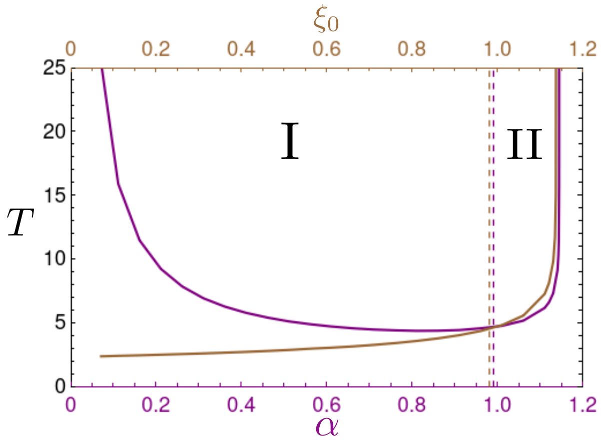


Figure S1: Time period, $T$ of shape oscillations in regions I and II as $\alpha$ (purple, $\xi_0 = 1$) and $\xi_0$ (brown, $\alpha = 1$) are varied.

## 3.2 Elongation and alignment angle in region III

In region III, the steady state of the system corresponds to deformed particles aligned at an angle to the shear, similar to the flow-aligned state of rigid liquid crystals. The extent of deformation, $r_s$, of the deformable particles subjected to a Couette flow is a function of $\alpha$ and $\xi_0$; it increases with both $\alpha$ and $\xi_0$ as shown in Fig. S2, but the dependence on $\xi_0$ is rather weak. The equilibrium alignment angle, $\theta_s$, of soft nematic particles differs from Leslie's angle for rigid nematic particles: $\theta_s = \frac{1}{2} \arccos\left(\frac{1}{\xi_0 r_s}\right)$ is dependent on the shear rate for the former, but it is independent of the shear rate for the latter.

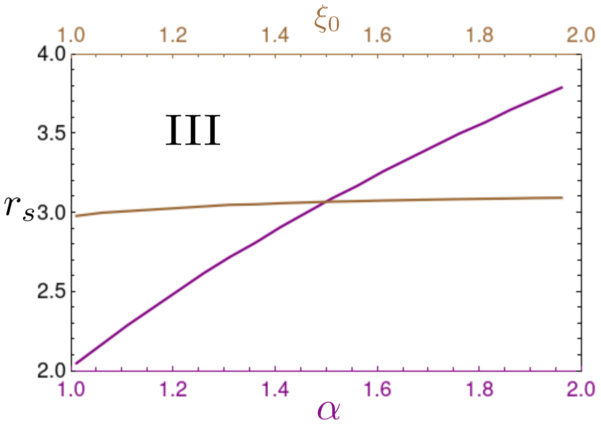


Figure S2: Extent of elongation of deformable particles, $r_s$ in region III as $\alpha$ (purple, $\xi_0 = 1.5$) and $\xi_0$ (brown, $\alpha = 1.5$) are varied.

### 3.3 Phase boundary of region I and minimum alignment angle

The phase boundary separating region I from region II in Fig. 1 can be determined analytically from the requirement that there exists exactly one solution to the steady-state of Eqs. (3) and (4), i.e. we require values of $\{\alpha, \xi_0\}$ such that the set of equations

$$\alpha(r_s + 1)\sin 2\theta_s - r_s\left(1 + \epsilon r_s^2\right) = 0, \tag{S1}$$

$$\frac{\alpha}{2}\left(\xi_0 r_s \cos 2\theta_s - 1\right) = 0, \tag{S2}$$

admits a unique solution for $\{r_s, \theta_s\}$. The solution to Eq. (S2) is given by $\cos 2\theta_s = 1/(\xi_0 r_s)$. Eliminating $\theta_s$, from Eq. (S1), we find an expression for $\alpha(r_s, \xi_0)$,

$$\alpha(r_s, \xi_0) = \frac{r_s\left(1 + \epsilon r_s^2\right)}{(r_s + 1)\sqrt{1 - 1/(\xi_0 r_s)^2}}. \tag{S3}$$

The dependence of $\alpha(r_s)$ for fixed values of $\xi_0$ is shown in Fig. S3. Clearly there is a minimum in the function $\alpha(r_s)$. For larger values of $\alpha$, there are two solutions: the smaller solution corresponds to the saddle point and the larger solution corresponds to the fixed point in the $\{r, \theta\}$ space. Below the minimum, there are no solutions, namely the saddle-node bifurcation does not occur. At the turning point, there is a unique solution for $r_s$. Calculating $d\alpha/dr_s = 0$, the resulting quintic equation is:

$$r_s(r_s(\xi_0^2 + \epsilon(r_s(r_s(3 + 2r_s)\xi_0^2 - 3) - 4)) - 1) - 2 = 0, \tag{S4}$$

which can be solved numerically to determine the value of $\alpha$ for which the unique solution exists for a given $\xi_0$. By varying $\xi_0$ and repeating this process, the full phase boundary for region I may be computed.

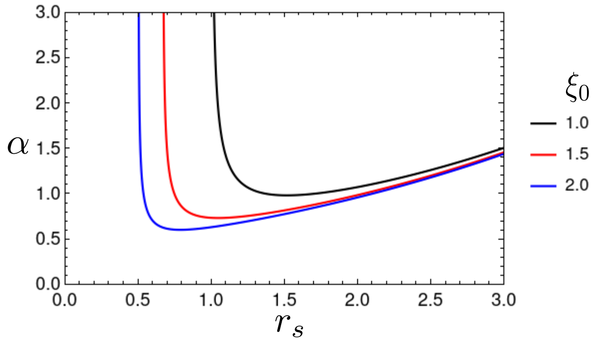


Figure S3: Plot of $\alpha(r_s)$ given by Eq. S3 for varying values of $\xi_0$. The turning point corresponds to the value of $\alpha$ with a unique solution for $r_s$.

This procedure also allows us to determine the value of $r_s$ and $\theta_s$ along the boundary separating region I from the rest of the phase diagram. These values correspond to the least elongation $r_s^m$ and the corresponding alignment angle $\theta_s^m$ at which the deformable nematics can flow align. The obtained values of $r_s^m$ and $\theta_s^m$ as a function of the flow-alignment scale $\xi_0$ are shown in Fig. S4.

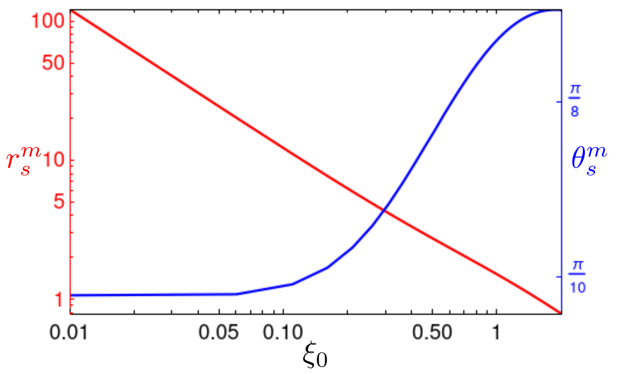


Figure S4: Minimum values of the extent of elongation $r_s^m$ (red curve) and the alignment angle $\theta_s^m$ (blue curve) of the flow aligning deformable particles as $\xi_0$ is varied. $\theta_s^m$ asymptotes to a constant as $\xi_0 \to 0$ showing that the minimum angle at which a deformable nematic flow-aligns never reaches zero.

$\theta_s^m$ decreases with decreasing $\xi_0$. We may arrive at an analytic expression for its asymptotic value by considering the behaviour of Eq. (S4) as $\xi_0 \to 0$ and $r_s^m \to \infty$, while their product remains finite. This is further motivated by the fact that Fig. S4 shows $r_s^m \sim 1/\xi_0$. Considering the relevant terms of Eq. (S4) we obtain,

$$\epsilon (r_s^m)^3 \left(2\xi_0^2 (r_s^m)^2 - 3\right) = 0, \tag{S5}$$

which has a non-zero solution of $r_s^m(\xi_0 \to 0) = \sqrt{3/2}/\xi_0$. Substituting this into Eq. (S2) gives $\theta_s^m(\xi_0 \to 0) = \frac{1}{2} \arccos \sqrt{2/3}$. This result shows that, within this model of deformable nematics, there is a non-zero minimum flow alignment angle. This is in contrast to rigid nematics which exhibit a minimum flow alignment angle of zero.

# 4 Dynamics of non-circular ($r_0 > 0$) particles in Couette flow

In the main manuscript we considered deformable nematics with a circular equilibrium shape, $r_0 = 0$. Here, we consider the case of a continuum of particles that inherently have an elongated shape, $r_0 > 0$. The phase-space diagram in this case is qualitatively similar to that of circular particles presented in Fig. 1. The three distinct regions I-III remain, but with their phase boundaries shifted to lower $\alpha$, and lower $\xi_0$, not necessarily by an equal amount. This shift arises because a flow aligned state can be maintained at lower shear rates as $r_0$ increases.

The steady states that the system achieves in regions II and III remain qualitatively the same, but the dynamics in region I becomes richer as tumbling trajectories become possible. Fig. S5 shows the phase space trajectories of a deformable nematic with an equilibrium shape of $r_0 = 1/2$ as $\alpha$ is varied. For $\alpha \ll 1$, the strain rate is too weak to deform the particles appreciably, but the vorticity component drives the rotation. Thus, the shape oscillations observed in region I remain, but with a small amplitude as shown in Fig. S5($a$) (bottom). Since the vorticity drives the particles to rotate through an angle $2\pi$, the limit cycle in phase space closely follows a circle of radius $r = r_0$ as shown in Fig. S5($a$) (top). The dynamics observed in this limit corresponds to the dynamics of rigid nematics with an effective Leslie flow-aligning parameter $\xi_0 r_0$.

As $\alpha$ is increased, the extent of elongation (for $\theta > 0$), and that of contraction (for $\theta < 0$) also increase. Though the tumbling motion persists, the trajectory in phase space is deformed into a

dumbbell (see Fig. S5$(b)$). At a critical value $\alpha_c(r_0)$, the trajectory reaches the origin of phase space, and the particles re-extend along $\theta = \pi/4$ giving qualitatively the same trajectories as for nematic particles with $r_0 = 0$.

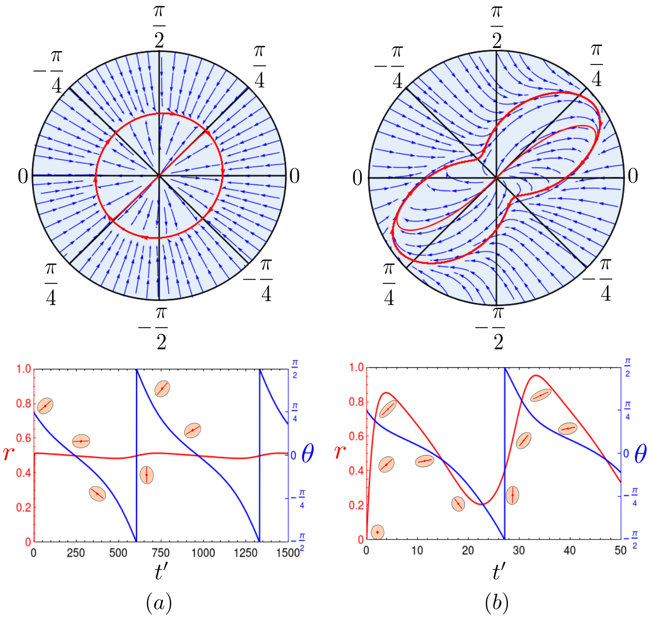

Figure S5: Shape oscillations and tumbling motion of inherently elongated ($r_0 > 0$), deformable nematics: temporal variation of $\{r(t'), \theta(t')\}$ (bottom) and the corresponding phase space trajectories in the $\{r, \theta\}$ space (top). $(a)$ $\alpha = 0.001 \ll 1$, where the limit of rigid nematics is recovered. $(b)$ $0 < \alpha = 0.25 < \alpha_c$ where the variation in particle deformation is more pronounced. Here, $\xi_0 = 1$. The red trajectories correspond to the initial conditions $\{0, \pi/4\}$.

# 5 Kymographs of $r(y', t')$ and $\theta(y', t')$ for $\beta \neq 0$

Fig. 4(a) in the manuscript illustrates the Kymograph showing spatio-temporal evolution, $r(y', t')$, of deformable nematics in a Poiseuille flow at $\beta = 0$. In Fig. S6, we present similar kymographs of $r$ and $\theta$ for $\alpha_p = 1.8$ but for $\beta = 0.05$. Neumann boundary conditions are applied for $\theta$ at the channel walls to perform these simulations. Inclusion of nematic elasticity ($\beta \neq 0$) results in further development of the spatial coherence in the microstructure of deformable particles. The dynamics continue to be time dependent with the central band expanding and contracting continuously, in addition to the tumbling dynamics of particles in the central band observed at $\beta = 0$. It may also be noted that the features associated with the temporal evolution of the central band seen in Fig. S6 are essentially similar to that in Fig. 4(b) in the manuscript where $\beta$ is changed stepwise.

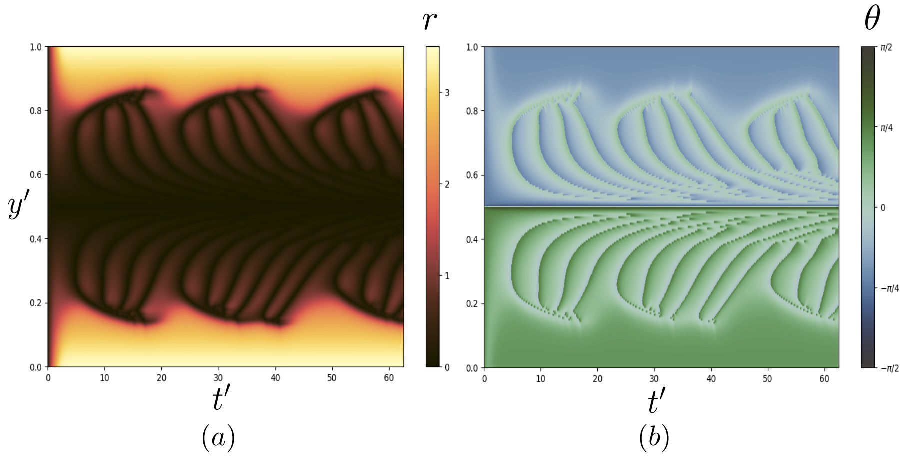


Figure S6: Kymographs of $(a)$ $r(y', t')$ and $(b)$ $\theta(y', t')$ in a Poiseuille flow for $\alpha_p = 1.8, \beta = 0.05$.

# 6 Variation of nematic order parameter in Couette and Poiseuille flows

In the manuscript, we have implicitly set the nematic order parameter to be constant. Here, we present how this specific limit arises and discuss what happens when the assumption of constant nematic order parameter is relaxed.

Consider the form of the free energy used in Ref. (34),

$$f = \frac{A_Q}{2}\left(S_{eq}^2 - \frac{2}{3}Q_{ij}Q_{ji}\right)^2 + \frac{K(r)}{2}\left(\partial_k Q_{ij}\right)^2.$$

Here, deviating from the classical Onsager calculation we choose $S_{eq} = r/(r+1)$, the value of $S$ that minimises the free energy. $S = 0$ for circular particles and $S \to 1$ as the aspect ratio of the deformed particles approaches $\infty$. Thus, for the case of Couette flow we obtain the following system of equations:

$$\dot{S} = \frac{8\kappa}{3}\left(S_{eq}^2 - S^2\right)S + r\xi_0\alpha\sin 2\theta\left(\frac{4}{9} + \frac{1}{3}S - \frac{3}{2}S^2\right) \tag{1}$$

$$\dot{r} = \alpha(r+1)\sin 2\theta - r\left(1 + \epsilon r^2\right) \tag{2}$$

$$\dot{\theta} = \frac{\alpha}{2}\left(\xi_0\frac{3S+4}{9S}r\cos 2\theta - 1\right), \tag{3}$$

where $\kappa = \Gamma A_Q/\left(\Gamma_r A_r\right)$ and we set $r_0 = 0$. In the limit $\Gamma A_Q \gg \xi_0\dot{\gamma}$, $S$ can be approximated as $S = S_{eq} = r/(r+1)$, reducing the number of ODEs to 2. The other limit $\Gamma A_Q \ll \xi_0\dot{\gamma}$ gives a constant $S = 2/3$.

We take the limit where $S = 2/3$ in the manuscript. However, we have performed numerical simulations for the other limit, where $S = S_{eq} = r/(r+1)$. We find that the same saddle-node bifurcation exists in the $r-\theta$ space, but, naturally, at different values of the variables and parameters. Fig. S7 shows the relevant phase space diagrams. It is clear that the qualitative results remain

unchanged. This is because, the main factor behind these results is the shape dependent flow-aligning parameter, a key point made in the main text. A phase diagram similar to Fig. 1 in the main text may be computed with only quantitative differences.

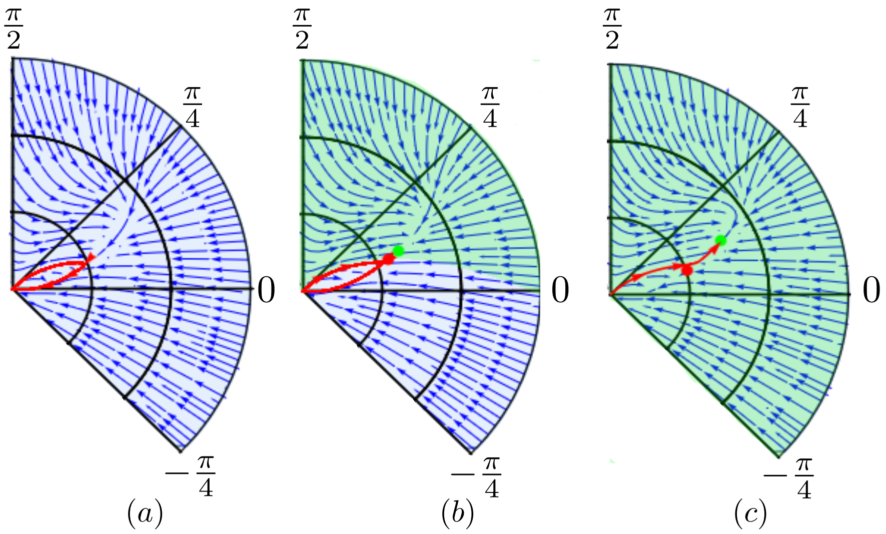


Figure S7: Phase space trajectories of the deformable nematics in $\{r, \theta\}$ space in the simplified case of $S = S_{eq}$, thus relaxing the assumption of constant $S$ in contrast to the results reported in the manuscript. Here, $\xi_0 = 1$ and $\alpha = \{0.85, 0.91, 0.95\}$ in $(a) - (c)$ respectively. Red trajectories correspond to the initial conditions $\{0, \pi/4\}$. Steady state $\{\dot{r} = 0, \dot{\theta} = 0\}$ solutions exist as saddle (red) and stable (green) points. Green background labels the basin of attraction for the stable point.

Given the above discussion, it is expected that $S$ only plays a quantitative role. We illustrate this by considering the following parameters: $r_0 = 0, \xi_0 = 1, \alpha = 0.8, \epsilon = 0.1$, which places the system in Region I of the phase diagram reported in the manuscript. We set initial conditions $r(0) = 0, \theta(0) = \pi/4, S(0) = 2/3$. The following three cases: $\Gamma A_Q/(\xi_0\dot{\gamma}) \ll 1, \approx 1$ and $\gg 1$ are considered. Fig. S8 shows the plots of $r(t), \theta(t), S(t)$ for the cases $\Gamma A_Q/(\xi_0\dot{\gamma}) = \{0.00125, 1.25, 125\}$ obtained by varying the value of $\kappa$. While $S(t)$ is now a dynamical variable, there is only a quantitative change in the plots between the different values of $\Gamma A_Q/(\xi_0\dot{\gamma})$. Unsurprisingly, these quantitative changes also translate to a shift in the phase boundaries of Fig. 1 in the manuscript. The qualitative form remains the same.

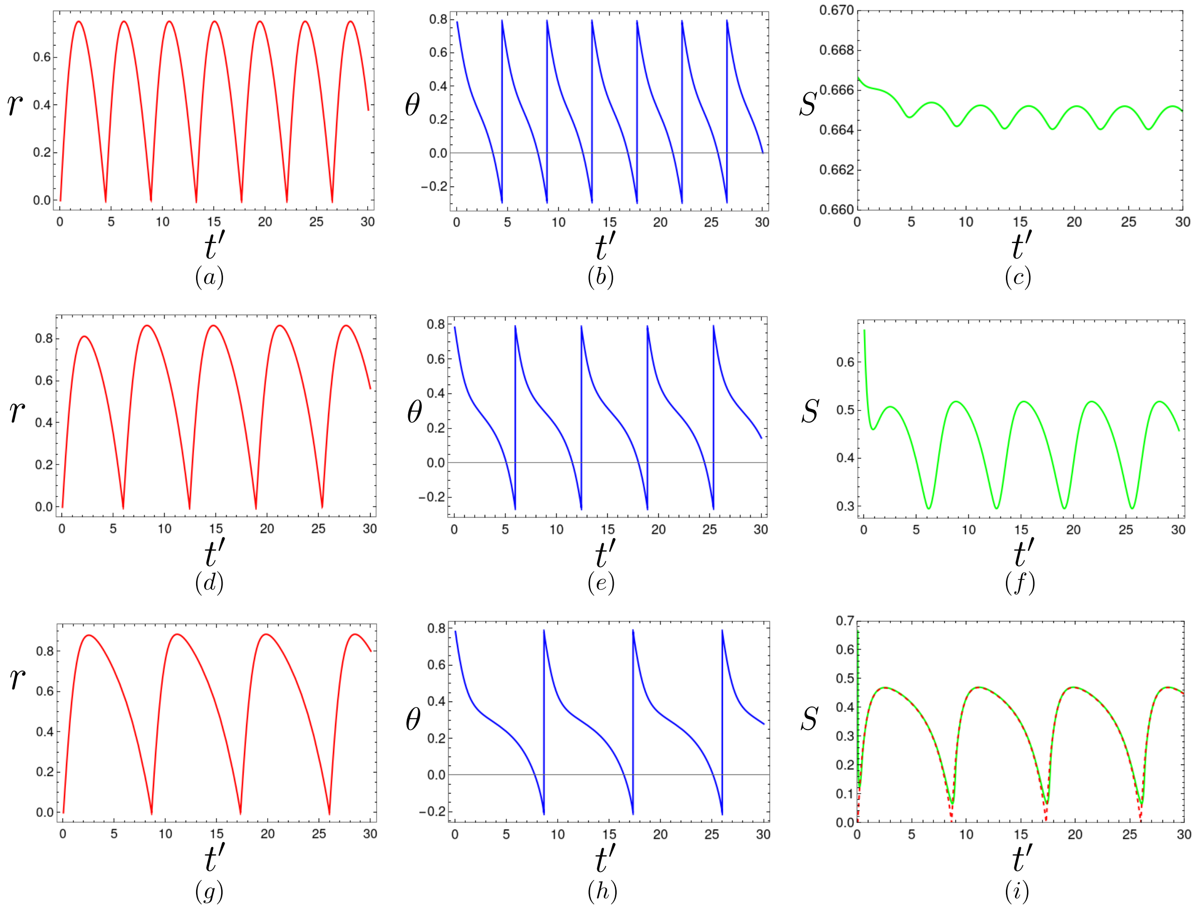


Figure S8: Time evolution of $r$ (red), $\theta$ (blue) and $S$ (green) for different values of the parameter $\kappa$. $(a)-(c)$ $(\Gamma A_Q/(\xi_0\dot{\gamma})) = 0.00125$. The value of $S$ oscillates very closely around 2/3, verifying the validity of the approximation $S = 2/3$ in this limit. $(d)-(f)$ $(\Gamma A_Q/(\xi_0\dot{\gamma})) = 1.25$, which corresponds to an intermediate regime where $r$ attains values of $\mathcal{O}\left(\Gamma A_Q/(\xi_0\dot{\gamma})\right)$. In this case, small quantitative changes can be seen. $(g)-(i)$ $(\Gamma A_Q/(\xi_0\dot{\gamma})) = 125$, corresponding to the limit $(\Gamma A_Q/(\xi_0\dot{\gamma})) \gg 1$. In $(i)$, the red dashed line corresponds to $S_{eq} = r/(r+1)$, verifying the validity of the approximation $S = r/(r+1)$ in this limit.

See also Fig. S9 for simulation results in a Poiseuille flow where the nematic order parameter is a function of particle aspect ratio, $S(r)$. The simulations in this limit are done with Péclet number, $\alpha_p = 1.8$ and the elasticity parameter $\beta = 0, 0.05$. These kymographs are to be compared with Fig. 4$(a)$ in the manuscript for which $S = 2/3$ and $\beta = 0$ and Fig. S6 for which $S = 2/3$ and $\beta = 0.05$ respectively. Clearly, as for the case of Couette flow, the choice of a varying nematic order parameter does not qualitatively change the results of the Poiseuille flow presented in the manuscript, as the dynamics primarily arises from the interplay of flow induced deformation and the reorientation kinematics of particles.

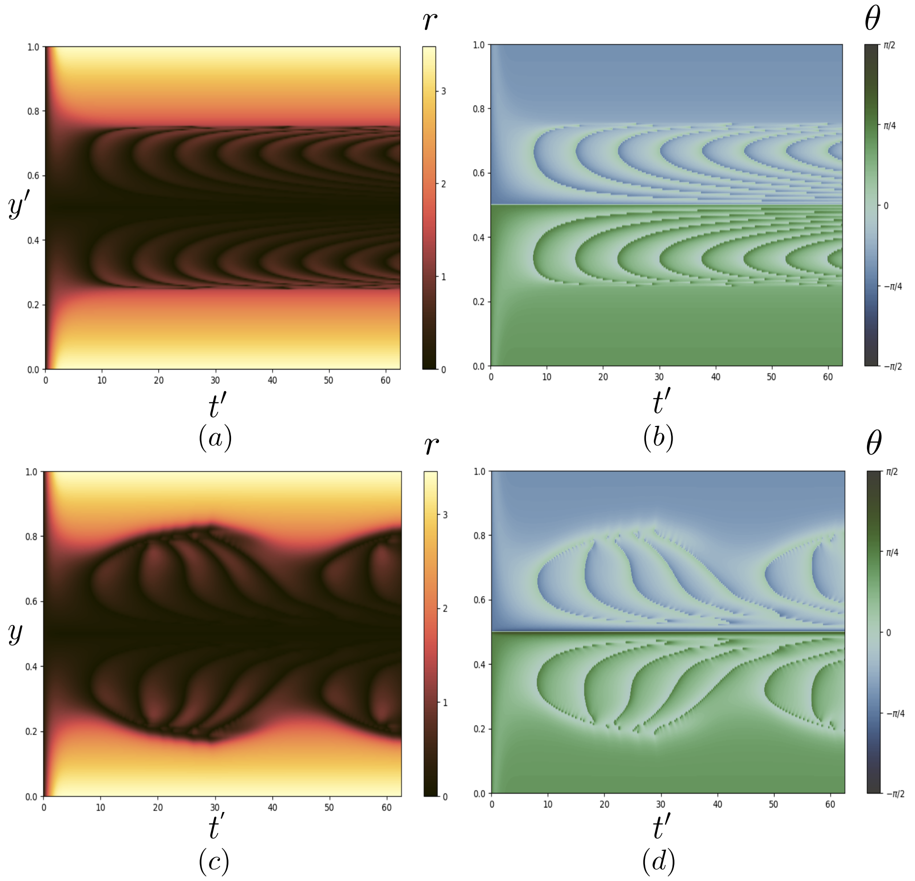


Figure S9: Kymographs of $r(y', t')$ and $\theta(y', t')$ in a Poiseuille flow where the nematic order parameter is given by $S(r) = r/(r+1)$. The simulations are for $\alpha_p = 1.8$, $(a)-(b)$ $\beta = 0$ and $(c)-(d)$ $\beta = 0.05$.

# 7 Complete expressions for molecular potential arising from the functional derivatives of the free energy $\mathcal{F}$

In the manuscript, only a minimal formulation arising from the free energy is retained in the expression for the molecular potential to keep the analysis simple. In this section, we present the full functional derivatives that contribute to Eqs. (5) and (6) in the main text. These read as:

$$\delta\mathcal{F}/\delta r = A_r(r - r_0) + A_r^*(r - r_0)^3 + \frac{K'(r)}{2}(\partial_{y'}\theta)^2, \tag{S6}$$

$$\delta\mathcal{F}/\delta\theta = -K(r)\partial_{y'}^2\theta - K'(r)(\partial_{y'}r)(\partial_{y'}\theta), \tag{S7}$$

where $K'(r) \equiv \partial K(r)/\partial r$. In the manuscript, the last terms in Eqs. S6 - S7 are omitted for simplicity. Including these terms does not change the results qualitatively. Fig. S10 shows kymographs of $r(y', t')$ and $\theta(y', t')$ for $\alpha_p = 1.8, \beta = 0.05$ in a Poiseuille flow, with the additional terms included.

Neumann boundary conditions are applied to both $r$ and $\theta$ on the channel walls. These figures are to be compared with Fig. S6. The complex spatio-temporal dynamics predicted in the manuscript, namely the wall-bound band of more elongated particles and the central band consisting of less elongated particles exhibiting patterns, are visible in both cases. The fact that the changes due to incorporation of the above terms are only quantitative is unsurprising, because these terms tend to suppress gradients of the $r$ and $\theta$ fields, leading to smoother profiles. However, the physics described in Fig. 1 of the manuscript remains unchanged.

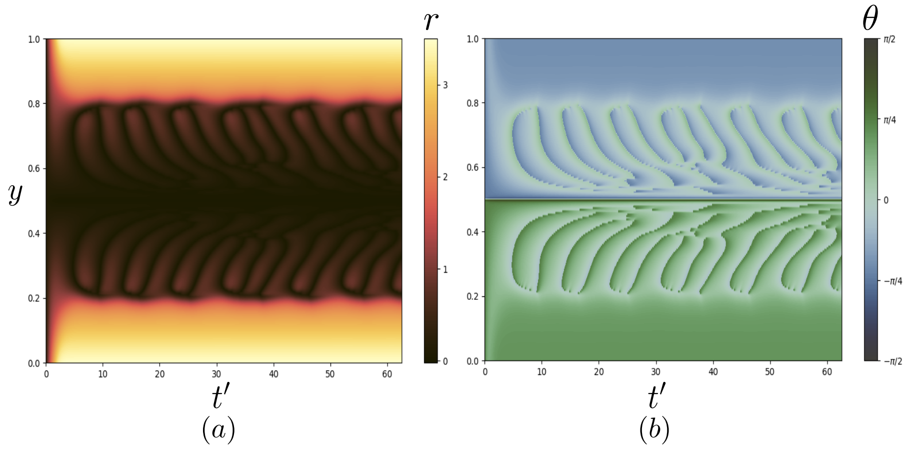


Figure S10: Kymographs of $(a)$ $r(y', t')$ and $(b)$ $\theta(y', t')$ of deformable nematics in a Poiseuille flow incorporating all terms described by Eq. S6-S7 into Eq. 5-6. Simulations are for $\alpha_p = 1.8, \beta = 0.05$.

# 8 Complete Navier-Stokes Model with Q tensor formalism

In this section we present generalized equations that describe the dynamical behavior of deformable nematic particles, accounting for the effect of stresses generated by the particles on the fluid flow.

The equation that governs the shape evolution of the particles is given by:

$$(\partial_t + u_i \partial_i)\, r = 2(r+1)E_{\parallel} - \Gamma_r \frac{\delta \mathcal{F}}{\delta r}, \tag{4}$$

where $u_i$ is the velocity field, $E_{ij}$ is the strain rate tensor, defined as the symmetric part of the velocity gradient tensor $\partial_i u_j$. $E_{\parallel} = n_i E_{ij} n_j$ is the projection of the strain rate, along the particles' orientation $n_i$ and $\frac{\delta \mathcal{F}}{\delta r} = A_r(r - r_0) + A_r^*(r - r_0)^3 + \frac{K'(r)}{2}(\partial_{y'}\theta)^2$, is the functional derivative of the free energy with respect to $r$. The ratio $A_r^*/A_r = \epsilon$ is the ratio of coefficients appearing in the first two terms in the expression for $\frac{\delta \mathcal{F}}{\delta r}$. Note that the additional terms from the free energy functional derivative mentioned in Section 7 are excluded for a closer comparison to the main manuscript's results.

The fluid flow is governed by the Navier-Stokes equations:

$$\partial_i u_i = 0\,, \tag{5}$$

$$\rho\left(\partial_t + u_k\partial_k\right)u_i = \partial_j\Pi_{ij}, \tag{6}$$

where $\rho$ is the fluid density and the stress tensor $\Pi_{ij}$ is given by

$$\Pi_{ij} = 2\eta E_{ij} - p\delta_{ij} - \xi(r)[H_{ik}\tilde{Q}_{kj} + \tilde{Q}_{ik}H_{kj} - 2\tilde{Q}_{ij}(Q_{kl}H_{lk})] + Q_{ik}H_{kj} - H_{ik}Q_{kj} - \partial_i Q_{kl}\left(\frac{\partial f}{\partial_j Q_{lk}}\right), \tag{7}$$

where $H_{ij} = -\delta\mathcal{F}/\delta Q_{ij} + (\delta_{ij}/3)\delta\mathcal{F}/\delta Q_{kk}$ is the molecular field, $\eta$ is the viscosity, $p$ is the bulk pressure and $\tilde{Q}_{ij} = \left(Q_{ij} + \frac{1}{3}\delta_{ij}\right)$, where $Q_{ij} = \dfrac{3S}{2}(n_i n_j - \dfrac{1}{3}\delta_{ij})$ is the nematic tensor order parameter in 3D which we constrain to lie on the 2D plane, *i.e* $n_z = 0$. The free energy density $f$ is chosen as:

$$f = \frac{A_Q}{2}\left(S_{eq}^2 - \frac{2}{3}Q_{ij}Q_{ji}\right)^2 + \frac{K(r)}{2}\left(\partial_k Q_{ij}\right)^2,$$

where $S_{eq}$ is the equilibrium value for the nematic order parameter $S$.

The Beris-Edwards equation of the nematic tensor $Q_{ij}$ is given by:

$$\left(\partial_t + u_k\partial_k\right)Q_{ij} - \mathcal{W}_{ij} = \Gamma H_{ij}, \tag{8}$$

where the generalized co-rotation term $\mathcal{W}_{ij}$ reads as:

$$\mathcal{W}_{ij} = \left(\xi(r)E_{ik} + \Omega_{ik}\right)\tilde{Q}_{kj} + \tilde{Q}_{ik}\left(\xi(r)E_{kj} - \Omega_{kj}\right) - 2\xi(r)\tilde{Q}_{ij}Q_{kl}W_{lk}, \tag{9}$$

where $W_{ij} = \partial_i u_j$ is the gradient of the velocity field and $\Omega_{ij} = (\partial_j u_i - \partial_i u_j)/2$ is the vorticity tensor.

The system of equations described above are solved using a hybrid lattice Boltzmann method. The following parameters are chosen for the simulations: lattice grid size $\Delta x = 1$ and time step size $\Delta t = 1$, $L = 200, \xi_0 = 1, G = 1.5 \times 10^{-5}, \eta = 2/3, \Gamma_r = 0.05, A_r = 0.025, A_r^* = 0.0025, A_Q = 0.4, S_{eq} = 2/3, \rho = 1$. The parameters are chosen to ensure that the dimensionless parameters $\alpha_p = 1.8$ and $\beta = 0.05$ are kept constant. Initial conditions were $r(y,0) = 0.1$ and $\theta(y,0) = \pm\pi/4$ for $y \lesseqgtr 100$ respectively, while the velocity field is initialized as a Poiseuille flow given by $u_x(y,0) = \dfrac{G}{2\eta}y(L-2y)$.

Further, we define Ericksen number $Er = \dfrac{\eta u_m L}{K_0}$ the ratio of viscous to elastic stresses that quantifies the role of elasticity. Here $u_m$ is the mean velocity across the channel width, and is equal to $GL^2/12\eta$ for a pure parabolic flow.

We consider the following two cases:

1. $\{\Gamma, K_0\} = \{12.625, 0.01\}$ that gives $Er = 1000$, thus yielding viscous stresses much greater than elastic stresses. The dynamics obtained are similar to the results presented in the manuscript. The results are illustrated using kymographs of the degree of elongation $r(y', t')$ and the angle of orientation $\theta(y', t')$ in Fig. S11($(a)-(b)$) and are to be compared with Fig. S6.

2. $\{\Gamma, K_0\} = \{2.525, 0.05\}$ that gives $Er = 200$, an intermediate value of the Ericksen number. In this case, elastic stresses become comparatively larger and the resulting velocity profile exhibits small deviations from the parabolic flow. The results are illustrated using kymographs of the degree of elongation $r(y', t')$ and the angle of orientation $\theta(y', t')$ in Fig. S11($(c)-(d)$). There is little qualitative change to the results even at this value of $Er$, namely the observations such as the existence of non-periodic shape oscillations across the channel and the enhanced flow-alignment for more elongated particles near the walls remain.

Thus, it is evident that the fully coupled system qualitatively reproduces the results presented in the manuscript, verifying the validity of the simple model. Moreover this analysis gives us an estimate of the range of $Er$ for which the assumption of imposed flow described in the main text is valid. Further investigation into lower Ericksen numbers require very high resolution lattice Boltzmann simulations, which would be very expensive in computer time.

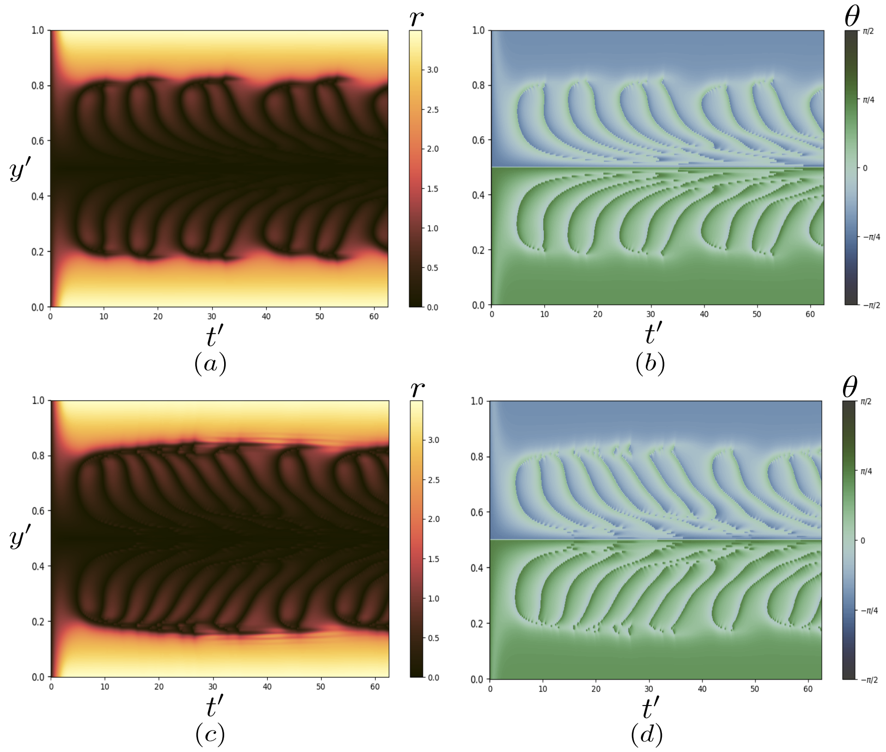


Figure S11: Kymographs of the degree of elongation, $r(y', t')$ and the angle of orientation $\theta(y', t')$, obtained using the full Navier-Stokes model with $\mathbf{Q}$ tensor formalism and solved using the hybrid lattice Boltzmann method. Simulations are run for $\alpha_p = 1.8, \beta = 0.05$ and for $(a) - (b)$ $Er = 1000$, and $(c) - (d)$ $Er = 200$, respectively.

## 9 Kymographs of $r(y', t')$ and $\theta(y', t')$ for varying $\beta$

In Fig. S12, we present kymographs of both the elongation, $r$ and the orientation $\theta$ as $\beta$ is varied in a step wise manner as in Figs. $4(b)$ and $4(c)$ in the main text.

## 10 Steady state dynamics of particles in Poiseuille flow

Fig. S13 shows the spatial variation of the steady-state solutions, $r_s(y')$ and $\theta_s(y')$ for $\alpha_p = 2, \beta = 0.25$ in Poiseuille flow, corresponding to a system deep in region B of Fig. $4(d)$. $\theta_s(y')$ reaches a constant value as it approaches the wall, to satisfy the boundary condition. Near the centre of

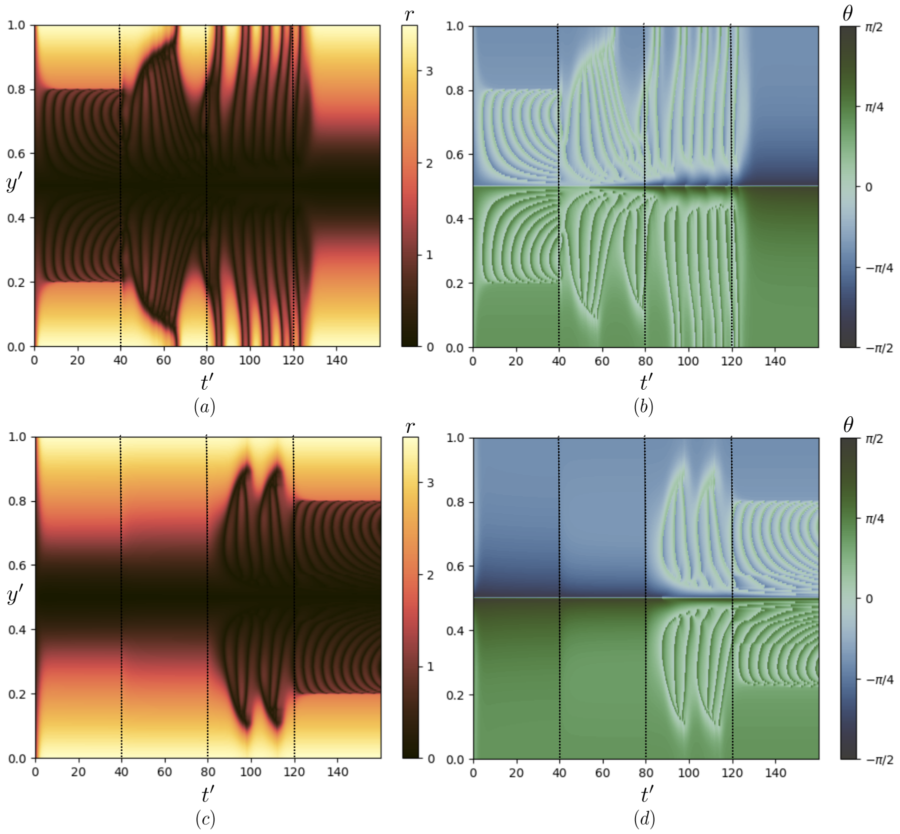


Figure S12: Kymographs of $(a)$ the degree of elongation $r(y', t')$ and $(b)$ the angle of orientation $\theta(y', t')$. Here $\alpha_p = 1.8$, and the simulation protocol is by varying $\beta$ in the range 0 and 0.3 in increments of 0.1 every 40 units of time. $(c) - (d)$ correspond to the backwards scenario where $\beta$ is reduced from 0.3 to 0.

the channel, the symmetry $\theta(y') = -\theta(y' + 1/2)$ enforces that $\theta_s \to \pm\pi/2$, resulting in a bend-like solution. These solutions may be obtained by solving the differential-algebraic system corresponding to $\dot{r} = 0, \dot{\theta} = 0$ in Eqs. (5) and (6).

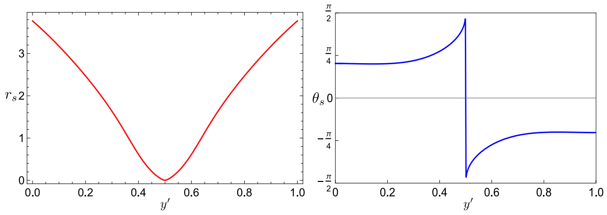


Figure S13: Steady state solutions, $r_s(y')$ and $\theta_s(y')$ for a system of deformable nematics with $\alpha_p = 2$, $\beta = 0.25$. The apparent discontinuity at $y' = 1/2$ in $\theta_s(y')$ is due to the nematic nature of the particles which automatically respects the equivalence of $\theta = \pm\pi/2$.

# References

[1] D. Koch, A. Nandan, G. Ramesan, I. Tyukin, A. Gorban, and A. Koseska, Phys. Rev. Lett. **133**, 047202 (2024).
